# Supplementary material for: The two-loop energy-momentum tensor within the gradient-flow formalism
Source: arXiv:1808.09837 ancillary file (2025-05-13)
Supplement: Supplementary file 1 [file MixingMatrix_Flavor.pdf]

# Supplement to Ref. [1]

R. Harlander, Y. Kluth, F. Lange

Here we describe the file `MixingMatrix_Flavor.m` which contains the mixing matrix between renormalized and flowed operators entering the flow-time definition of the energy-momentum tensor.

## 1 Mixing matrix

The mixing matrix  $\Omega_{ij}(t)$  defined in Eq. (25) of Ref. [1] distinguishes different quark flavors, i.e. the indices run over  $\{1, 2, 3_1, \dots, 3_{n_F}, 4_1, \dots, 4_{n_F}\}$ . Following the procedure of Sect. 7, we can express the renormalized QCD operators in terms of flowed operators without summing over the flavors by

$$\{\hat{\mathcal{O}}_i\}_R(x) = Z_{F,ij} H_{F,jk} \Omega_{kl}^{-1}(t) \tilde{\mathcal{O}}_l(t, x) \equiv M_{F,il}(t) \tilde{\mathcal{O}}_l(t, x), \quad (1)$$

where all matrices distinguish between the quark flavors and, thus,  $Z_{F,ij} \neq Z_{ij}$  of Eq. (59). Similar to  $\Omega_{ij}(t)$ ,  $M_{F,ij}(t)$  can be expressed as

$$M_F = \begin{pmatrix} M_{F,11} & M_{F,12} & \overline{M_{F,13}}^T & \overline{M_{F,14}}^T \\ M_{F,21} & M_{F,22} & \overline{M_{F,23}}^T & \overline{M_{F,24}}^T \\ \underline{M_{F,31}} & \underline{M_{F,32}} & \underline{\underline{M_{F,33}}} & \underline{\underline{M_{F,34}}} \\ \underline{\underline{M_{F,41}}} & \underline{\underline{M_{F,42}}} & \underline{\underline{M_{F,43}}} & \underline{\underline{M_{F,44}}} \end{pmatrix} \quad (2)$$

with

$$M_{F,ij} = m_{F,ij} \quad \text{for } i, j < 3, \quad (3)$$

$$\underline{M_{F,ij}} = m_{F,ij} \begin{pmatrix} 1 \\ \vdots \\ 1 \end{pmatrix} \quad \text{for } i < 3, j > 2 \quad \text{or } i > 2, j < 3, \quad (4)$$

$$\underline{\underline{M_{F,ij}}} = \begin{pmatrix} m_{F,ij} & \overline{m_{F,ij}} & \overline{m_{F,ij}} & \dots & \overline{m_{F,ij}} \\ \overline{m_{F,ij}} & m_{F,ij} & \overline{m_{F,ij}} & \dots & \overline{m_{F,ij}} \\ \overline{m_{F,ij}} & \overline{m_{F,ij}} & m_{F,ij} & \dots & \overline{m_{F,ij}} \\ \vdots & \vdots & \vdots & \ddots & \vdots \\ \overline{m_{F,ij}} & \overline{m_{F,ij}} & \overline{m_{F,ij}} & \dots & m_{F,ij} \end{pmatrix} \quad \text{for } i, j > 2. \quad (5)$$

Inserting these definitions into Eq. (1), we find for the renormalized QCD operators

$$\begin{aligned} \{\hat{\mathcal{O}}_i\}_R(x) = & m_{F,i1}(t) \tilde{\mathcal{O}}_1(t, x) + m_{F,i2}(t) \tilde{\mathcal{O}}_2(t, x) \\ & + m_{F,i3}(t) \tilde{\mathcal{O}}_3(t, x) + m_{F,i4}(t) \tilde{\mathcal{O}}_4(t, x) \quad \text{for } i = 1, 2 \end{aligned} \quad (6)$$

and

$$\begin{aligned} \{\hat{\mathcal{O}}_{i_f}\}_R(x) = & m_{F,i1}(t) \tilde{\mathcal{O}}_1(t, x) + m_{F,i2}(t) \tilde{\mathcal{O}}_2(t, x) \\ & + m_{F,i3}(t) \tilde{\mathcal{O}}_{3_f}(t, x) + m_{F,i4}(t) \tilde{\mathcal{O}}_{4_f}(t, x) \\ & + \sum_{f' \neq f} \left[ \bar{m}_{F,i3}(t) \tilde{\mathcal{O}}_{3_{f'}}(t, x) + \bar{m}_{F,i4}(t) \tilde{\mathcal{O}}_{4_{f'}}(t, x) \right] \quad \text{for } i = 3, 4, \end{aligned} \quad (7)$$

where

$$\tilde{\mathcal{O}}_i(t, x) = \sum_f \tilde{\mathcal{O}}_{i_f}(t, x) \quad \text{for } i = 3, 4. \quad (8)$$

The  $4 \times 4$  matrices  $m_F$  and  $\bar{m}_F$  can be found in the file `MixingMatrix_Flavor.m`.

Note that they are related to the mixing matrix  $Z_{ij} H_{jk} \zeta_{kl}^{-1}(t) \equiv M_{il}$  described in Ref. [1] by

$$M_{ij} = m_{F,ij} \quad \text{for } i < 3, \quad (9)$$

$$M_{ij} = n_F m_{F,ij} \quad \text{for } i > 2, j < 3, \quad (10)$$

$$M_{ij} = m_{F,ij} + (n_F - 1) \bar{m}_{F,ij} \quad \text{for } i > 2, j > 2. \quad (11)$$

## References

- [1] R. V. Harlander, Y. Kluth and F. Lange, *The two-loop energy-momentum tensor within the gradient-flow formalism*, Eur. Phys. J. C **78** (2018) no.11, 944 doi:10.1140/epjc/s10052-018-6415-7 [arXiv:1808.09837 [hep-lat]].
